# Supplementary material for: Kinematic analysis of the super-extended HI disk of the nearby spiral galaxy M83
Source: arXiv:2304.02037 source file (2023-04-04)
Supplement: Supplementary file 1 [file table-appendix.tex]

{

\begin{table*}[]
\centering
\caption{Properties of environmental regions in \gal. \textcolor{red}{\bf Similar to \autoref{tab:regions} but here we show the range of each quantity (i.e. minimum and maximum) for each region.}}
\label{tab:regions_appendix}
\begin{tabular}{lcccccc}
\hline \hline
\multicolumn{1}{c}{} &  $I_{\rm HI}$ &  $N_{\rm HI}$ &  \sigatom  &  \sigeff  &  \vlos  &  \vres   \\
\multicolumn{1}{c}{\multirow{-2}{*}{Region}} & [K km s$^{-1}$]& [$10^{20}$~cm$^{-2}$] & [M$_{\odot}$ pc$^{-2}$] & [km s$^{-1}$] & [km s$^{-1}$] & [km s$^{-1}$]   \\
\multicolumn{1}{c}{\multirow{1}{*}{(1)}} & (2) & (3) & (4) & (5) & (6) & (7)  \\
\hline
central disk & 
$46.2 - 837.1$&
$0.8 - 15.2$&
$0.7 - 12.6$&
$4.3 - 22.9$&
$420.3 - 628.3$&
$-47.5 - 44.5$
\\
ring & 
$40.4 - 565.4$&
$0.7 - 10.3$&
$0.6 - 8.5$&
$3.7 -22.5$&
$374.1 - 646.4$&
$-44.2 - 49.6$
\\
southern area &
$28.5 - 403.7$&
$0.5 - 7.4$&
$0.4 - 6.1$&
$2.4 -19.3$ &
$522.9 - 652.4$&
$-40.4 - 39.3$
\\
southern arm &
$37.1 - 310.9$&
$0.7 - 5.7$& 
$0.6 - 4.7$&
$1.5 - 17.7$  &
$414.6 - 639.0$&
$-47.1 - 23.4$
\\
northern arm &
$27.0 - 319.2$&
$0.5 - 5.8$&
$0.4 - 4.8$&
$2.5 - 19.2$ &
$363.5 - 650.7$&
$-49.6 - 43.0$
\\
\hline 
\end{tabular}
 \begin{minipage}{2.0\columnwidth}
        \vspace{1mm}
        {\bf Notes.} (1): Defined environmental regions in \gal: central disk, ring, southern area, southern and northern arm. (2--8): We show the range of values of each quantity for each region. (2): \hi\ integrated intensity. (3): \hi\ column density. (4): \hi\ surface density. (5): \hi\ effective line width. (6): L.o.s velocity. (7): Residual velocity. 
    \end{minipage}
\end{table*}}
